# Supplementary material for: Rethinking Round-Trip Translation for Machine Translation Evaluation
Source: arXiv:2209.07351 source file (2026-11-13)
Supplement: Supplementary file 1 [file wmt20_news_appendix.tex]

\begin{table}[ht]
\centering
\resizebox{1.0\linewidth}{!}{
\begin{tabular}{l| cc|cc}
\hline
\multirow{2}{*}{\textbf{Langauge Pair}} & \multicolumn{2}{c|}{\textbf{Pearson's} $\boldsymbol r$ $\uparrow$} & \multicolumn{2}{c}{\textbf{Kendall's} $\boldsymbol \tau$ $\uparrow$} \\
% & cs-en & de-en &de-fr  & en-cs  & en-de  & en-ru & en-zh & fr-de  & ru-en  & zh-en & average \\
\cline{2-5}
& \textbf{Our} & \comet & \textbf{Our} & \comet\\
\hline
 cs-en  &0.91 & 0.95 &0.60 & 0.60 \\
de-en  &0.95 & 0.75&0.80 & 0.20 \\
de-fr &0.97 & 0.70&0.80 & 0.80 \\
en-cs &0.94& 0.90&0.60 & 0.80 \\
en-de &0.92 &0.78 &1.00 & 0.40 \\
en-ru &0.85& 0.91&0.40 & 1.00 \\
en-zh &0.80 & 0.91& 0.80 & 0.80\\
fr-de &0.94& 0.92& 1.00 & 0.80\\
ru-en &0.85& 0.71&0.80 & 0.40\\
zh-en &0.50& 0.53& 0.20 & 0.40\\
\hline
Average  & \textbf{0.86} & 0.81 & \textbf{0.70} & 0.62 \\
\hline
\end{tabular}
}
\caption{Comparison of our predictors and \comet on ranking the translation quality of the selected MT systems on \wmtnews shared tasks.}
\label{tab:wmt20news_results_appendix}
\end{table}
